# Supplementary material for: A theory of the dark matter
Source: arXiv:2203.12405 ancillary file (2022-03-24)
Supplement: Supplementary file 1 [file Arithmetic_and_algebra.pdf]

# Arithmetic and algebra

This SageMath notebook does arithmetic and algebra for the paper *A theory of the dark matter*.

The section numbering follows the paper. Equation numbers refer to equations in the paper.

## Preamble

Code for displaying equations.

```
In [1]: %display latex
LE = lambda latex_string: LatexExpr(latex_string);
```

The numerical values of fundamental constants and basic physical quantities are stored in the dictionary `value[]`.

Physical units such as 's' and 'GeV' are defined as algebraic variables.

The dictionary `formula[]` will contain the formulas for derived physical quantities. For example, `formula[kappa] = 8*pi*G`.

The function `valof(x)` substitutes in a formula `x` to obtain a numerical value.

The function `print_values(x1,x2,...)` prints formulas `xn` with their numerical values.

```
In [2]: value = {}
formula={}
```

```
In [3]: def valof(x):
    SymRing = FractionField(PolynomialRing(RR, 's,GeV,J,m,kg,K,C'))
    NumRing = FractionField(PolynomialRing(RDF, 's,GeV,J,m,kg,K,C'))
    xval = SR(x)
    for a in reversed(formula):
        xval = xval.subs({a:formula[a]})
    for key,val in value.items():
        xval = xval.subs({key:val})
    xval = NumRing(xval)
    return xval
def print_values(*args):
    print_list=[]
    for arg in args:
        if arg in formula:
            print_list += [arg, '=', formula[arg], '=', valof(arg), LE(r'\qquad')]
        else:
            print_list += [arg, '=', valof(arg), LE(r'\qquad')]
    print_list.pop()
    pretty_print(*print_list)
```

## 1.3 Physical parameters

### Units and fundamental constants as variables

declare units as variables

```
In [4]: s = var('s', domain='positive', latex_name='\\mathrm{s}'); assume(s, 'real');
GeV = var('GeV', domain='positive', latex_name='\\mathrm{GeV}'); assume(GeV, 'real');
J = var('J', domain='positive', latex_name='\\mathrm{J}'); assume(J, 'real');
m = var('m', domain='positive', latex_name='\\mathrm{m}'); assume(m, 'real');
kg = var('kg', domain='positive', latex_name='\\mathrm{kg}\\,'); assume(kg, 'real');
K = var('K', domain='positive', latex_name='\\mathrm{K}'); assume(K, 'real');
C = var('C', domain='positive', latex_name='\\mathrm{C}'); assume(C, 'real');
km = var('km', domain='positive', latex_name='\\mathrm{km}\\,'); assume(km, 'real');
Mpc = var('Mpc', domain='positive', latex_name='\\mathrm{Mpc}\\,'); assume(Mpc, 'real');
```

declare fundamental constants and physical parameters as variables

```
In [5]: # fundamental constants
c = var('c', latex_name=r" c ")
c_mps = var('c_mps', latex_name=r" c ")
e_charge = var('e_charge', latex_name=r" e ")
```

```

hbar = var('hbar', latex_name=r"\hbar")
kB = var('kB', latex_name=r"k_{B}")
G = var('G', latex_name=r"G")
kappa = var('kappa', latex_name=r"\kappa")
#
# numbered constants c_n for temporary use
# c_ = var('c_', n=20, latex_name=r"c")
#
# Standard Model
GFermi = var('GFermi', latex_name=r"G_{\mathrm{Fermi}}")
m_W = var('m_W', latex_name=r"m_{W}")
m_Higgs = var('m_Higgs', latex_name=r"m_{\mathrm{Higgs}}")
hbar_v = var('hbar_v', latex_name=r"\hbar v")
v = var('v', latex_name=r"v")
g = var('g', latex_name=r"g")
lambdaH = var('lambdaH', latex_name=r"\lambda")
#
# cosmological parameters
H0 = var('H0', latex_name=r"H_{0}")
Omega_curvature = var('Omega_curvature', latex_name=r"\Omega_{\mathrm{curvature}}")
Omega_Lambda = var('Omega_Lambda', latex_name=r"\Omega_{\Lambda}")
#
# time and energy scales
t_grav = var('t_grav', latex_name=r"t_{\mathrm{grav}}")
t_Higgs = var('t_Higgs', latex_name=r"t_{\mathrm{Higgs}}")
t_Hubble = var('t_Hubble', latex_name=r"t_{\mathrm{Hubble}}")

```

## Values of the fundamental constants from NIST 2018

```

In [6]: value[G]          = 6.67430e-11*m^3*kg^(-1)* s^(-2)
value[e_charge] = 1.602176634e-19 * C
value[c]=c_mps  = 2.99792458e8 * m * s^(-1)
value[hbar]     = 1.054571817e-34*J*s
value[kB]       = 1.380649e-23*J*K^(-1)

```

```

In [7]: print_values(G,e_charge,c)
print('\n')
print_values(hbar,kB)

```

$$G = \frac{6.6743 \times 10^{-11} m^3}{s^2 kg} \quad e = 1.602176634 \times 10^{-19} C \quad c = \frac{299792458.0 m}{s}$$

$$\hbar = 1.054571817 \times 10^{-34} sJ \quad k_B = \frac{1.380649 \times 10^{-23} J}{K}$$

The constant  $\kappa = 8\pi G$ .

```

In [8]: formula[kappa] = 8*pi*G
print_values(kappa)

```

$$\kappa = 8\pi G = \frac{1.6774345478283484 \times 10^{-09} m^3}{s^2 kg}$$

convert to c=1 units with unit of energy = GeV

```

In [9]: conv={}
conv[m]  = c^(-1)*m
conv[kg] = J*s^2*m^(-2)
conv[J]  = e_charge^(-1) * C * 1e-9 * GeV
for a,b in conv.items():
    value[a] = a.subs(conv).subs(value)
#
print_values(c,J)
print('\n')
print_values(m,kg)
print('\n')
print_values(hbar,kB)

```

```
print('\n')
print_values(G,kappa)
```

$$c=1.0 \quad J=6241509074.460764 \text{ GeV}$$

$$m=3.3356409519815204 \times 10^{-09} s \quad kg=5.6095886038044526 \times 10^{26} \text{ GeV}$$

$$\hbar=6.582119565476076 \times 10^{-25} s \text{ GeV} \quad k_B=\frac{8.61733326214518 \times 10^{-14} \text{ GeV}}{K}$$

$$G=\frac{4.415832614329417 \times 10^{-63} s}{\text{GeV}} \quad \kappa=8 \pi G=\frac{1.1098197840527606 \times 10^{-61} s}{\text{GeV}}$$

## Standard Model coupling constants from PDG (2020, 2021)

measured quantities

```
In [10]: value[G_Fermi] = 1.1663787e-5*GeV^(-2);
value[m_W] = 80.379*GeV;
value[m_Higgs] = 125.10*GeV;
#
print_values(G_Fermi,m_W,m_Higgs)
```

$$G_{\text{Fermi}}=\frac{1.1663787 \times 10^{-05}}{\text{GeV}^2} \quad m_W=80.379 \text{ GeV} \quad m_{\text{Higgs}}=125.1 \text{ GeV}$$

derived quantities

```
In [11]: #
formula[hbar_v] = 2^(-1/4)*G_Fermi^(-1/2)
formula[v] = formula[hbar_v]/hbar
formula[g] = 2*m_W/hbar_v;
formula[lambaH] = m_Higgs/hbar_v;
#
print_values(hbar_v,v)
print('\n')
print_values(g,g^2)
print('\n')
print_values(lambaH,lambaH^2)
```

$$\hbar v=\frac{2^{\frac{3}{4}}}{2 \sqrt{G_{\text{Fermi}}}}=246.2196507941374 \text{ GeV} \quad v=\frac{2^{\frac{3}{4}}}{2 \sqrt{G_{\text{Fermi}}}\hbar}=\frac{3.740735007087775 \times 10^{26}}{s}$$

$$g=\frac{2 m_W}{\hbar v}=0.6529048330687819 \quad g^2=0.4262847210445737$$

$$\lambda=\frac{m_{\text{Higgs}}}{\hbar v}=0.5080829235055462 \quad \lambda^2=0.25814825715794265$$

## Cosmological parameters

units of distance

The value of 1 parsec in meters is taken from *IAU 2015 Resolution B2*, note 4 which references the definition as exactly  $64000/\pi$  au and the definition of au from *IAU 2012 Resolution B2*.

```
In [12]: value[km] = 1e3 * m
value[Mpc] = 1e6 * 3.085677581 * 1e16 * m
print_values(km,Mpc)
```

$$\text{km}=1000.0m \quad \text{Mpc}=3.0856775810000003 \times 10^{22}m$$

From Particle Data Group 2020 Particle Physics Booklet

```
In [13]: formula[H0] = 6.74e1 * km * s^(-1) * Mpc^(-1)
value[Omega_curvature] = 0.001
value[Omega_Lambda] = 0.685
#
print_values(H0, Omega_Lambda, Omega_curvature)
```

$$H_0 = \frac{67.40000000000000 \text{ km}}{\text{Mpc s}} = \frac{2.1842852414333302 \times 10^{-18}}{s} \quad \Omega_\Lambda = 0.685 \quad \Omega_{\text{curvature}} = 0.001$$

## time and energy scales

```
In [14]: formula[t_grav] = sqrt(kappa*hbar)
formula[t_Higgs] = hbar/m_Higgs
formula[t_Hubble] = 1/H0
#
print_values(t_grav, hbar/t_grav)
print('\n')
print_values(t_Higgs, m_Higgs)
print('\n')
print_values(t_Hubble, hbar/t_Hubble)
```

$$t_{\text{grav}} = \sqrt{\hbar \kappa} = 2.7027701557413476 \times 10^{-43} s \quad \frac{\hbar}{t_{\text{grav}}} = 2.435323459338203 \times 10^{18} \text{ GeV}$$

$$t_{\text{Higgs}} = \frac{\hbar}{m_{\text{Higgs}}} = 5.2614864632102925 \times 10^{-27} s \quad m_{\text{Higgs}} = 125.1 \text{ GeV}$$

$$t_{\text{Hubble}} = \frac{1}{H_0} = 4.5781566483679526 \times 10^{17} s \quad \frac{\hbar}{t_{\text{Hubble}}} = 1.4377226624218956 \times 10^{-42} \text{ GeV}$$

## 2.2 Initial CGF energy

elliptic parameter  $k_{\text{EW}}^2 = \frac{1}{2}$  and elliptic integral of first kind  $K_{\text{EW}} = K(k_{\text{EW}}) = K'(k_{\text{EW}})$

```
In [15]: # elliptic modulus and integrals
ksq_EW = var('ksq_EW', latex_name=r"k^2_{\mathrm{EW}}")
k_EW = var('k_EW', latex_name=r"k_{\mathrm{EW}}")
K_EW = var('K_EW', latex_name=r"K_{\mathrm{EW}}")
Kp_EW = var('Kp_EW', latex_name=r"K'_{\mathrm{EW}}")
#
value[ksq_EW] = 1/2
value[k_EW] = sqrt(1/2)
value[K_EW] = elliptic_kc(0.5)
value[Kp_EW] = elliptic_kc(0.5)
print_values(ksq_EW, K_EW, Kp_EW)
```

$$k_{\text{EW}}^2 = 0.5 \quad K_{\text{EW}} = 1.8540746773013719 \quad K'_{\text{EW}} = 1.8540746773013719$$

## 2.4 Start of the electroweak transition at $a = a_{\text{EW}}$

```
In [16]: a_EW = var('a_EW', latex_name=r"a_{\mathrm{EW}}")
#
a_EW_coeff = (6*pi)^(1/2)/(4*K_EW)
formula[a_EW] = a_EW_coeff * t_Higgs
print_values(a_EW_coeff, a_EW)
```

$$\frac{\sqrt{6}\sqrt{\pi}}{4 K_{EW}}=0.5854143283037644 \quad a_{EW}=\frac{\sqrt{6}\sqrt{\pi}t_{Higgs}}{4 K_{EW}}=3.0801495637396022 \times 10^{-27} s$$

```
In [17]: ahat_EW = var('ahat_EW', latex_name=r"\hat a_{\mathrm{EW}}")
formula[ahat_EW] = a_EW/t_Higgs
print_values(ahat_EW)
```

$$\hat{a}_{EW}=\frac{a_{EW}}{t_{Higgs}}=0.5854143283037644$$

## 2.6 Realizing the electroweak transition

```
In [18]: asqHsq_EW = var('asqHsq_EW', \
    latex_name=r"a_{\mathrm{EW}}^2 H_{\mathrm{EW}}^2+\epsilon^2")
formula[asqHsq_EW] = (t_grav^2/t_Higgs^2) * ( (1/(24*lambdaH^2))\
    * (a_EW^2/t_Higgs^2) + (1/(8*g^2)) * (t_Higgs^2/a_EW^2) )
print_values(asqHsq_EW)
print('\n')
expr = (t_grav^2/t_Higgs^2)/(4*sqrt(3)*g*lambdaH)
print_values(expr)
```

$$a_{EW}^2 H_{EW}^2 + \epsilon^2 = \frac{t_{grav}^2 \left( \frac{a_{EW}^2}{\lambda^2 t_{Higgs}^2} + \frac{3 t_{Higgs}^2}{a_{EW}^2 g^2} \right)}{24 t_{Higgs}^2} = 2.4037614729587787 \times 10^{-33}$$

$$\frac{\sqrt{3} t_{grav}^2}{12 g \lambda t_{Higgs}^2} = 1.1481436122987478 \times 10^{-33}$$

## 4.5 Parametrize the time evolution by $k^2$

```
In [19]: PSR.<k> = PowerSeriesRing(SR)
K_ps = (pi/2)*(1+k^2/4 + 9*k^4/64)+O(k^6)
E_ps = (pi/2)*(1-k^2/4 - 3*k^4/64)+O(k^6)
```

```
In [20]: alpha3 = (2*(1-k^2)*K_ps + 2*(2*k^2-1)*E_ps)/K_EW
pretty_print(LE(r"\alpha^3 = "), alpha3+O(k^4))
```

$$\alpha^3 = \frac{3\pi}{2 K_{EW}} k^2 + O(k^4)$$

```
In [21]: alpha2_b2 = k^2 - 1 + E_ps/K_ps; pretty_print(LE(r"\alpha^2 \langle b^2 \rangle = "), alpha2_b2+O(k^4))
```

$$\alpha^2 \langle b^2 \rangle = \frac{1}{2} k^2 + O(k^4)$$

```
In [22]: alpha2_mu2 = 1-2*k^2; pretty_print(LE(r"\alpha^2 \mu^2 = "), alpha2_mu2+O(k^2))
```

$$\alpha^2 \mu^2 = 1 + O(k^2)$$

```
In [23]: alpha4_E_CGF = k^2*(1-k^2)/2; pretty_print(LE(r"\alpha^4 E_{CGF} = "), alpha4_E_CGF+O(k^4))
```

$$\alpha^4 E_{CGF} = \frac{1}{2} k^2 + O(k^4)$$

```
In [24]: alpha2_ahat2 = (3/2)* alpha2_b2 + (4*lambdaH^2/g^2)* alpha2_mu2
```

```
pretty_print(LE(r"\alpha^2 \hat{a}^2= "),alpha2_ahat2+O(k^2))
```

$$\alpha^2 \hat{a}^2 = \frac{4\lambda^2}{g^2} + O(k^2)$$

```
In [25]: rhohat_CGF = (3*alpha4_E_CGF/g^2 +9*alpha2_b2^2/(32*lambdaH^2))/alpha2_ahat2^2
pretty_print(LE(r"\hat{\rho}_{CGF} = "),rhohat_CGF +O(k^4))
```

$$\hat{\rho}_{CGF} = \frac{3g^2}{32\lambda^4}k^2 + O(k^4)$$

```
In [26]: phat_CGF = ((alpha4_E_CGF-alpha2_mu2*alpha2_b2)/g^2 -9*alpha2_b2^2/(32*lambdaH^2))/alpha2_ahat2^2
pretty_print(LE(r"\hat{p}_{CGF} = "),phat_CGF +O(k^6))
```

$$\hat{p}_{CGF} = \left( \frac{9g^4 \left( \frac{8}{g^2} - \frac{1}{\lambda^2} \right)}{2048\lambda^4} \right) k^4 + O(k^6)$$

## 5.1 $\Omega_{CGF} + \Omega_{\Lambda} = 1$

```
In [27]: k0sq = var('k0sq',latex_name=r"k_{0}^{2}")
expr = t_Higgs^4/(t_grav^2*t_Hubble^2)*(32*lambdaH^4/g^2)
formula[k0sq] = 0.315*expr
pretty_print(k0sq,LE(' = 0.315 '),expr,'=',valof(k0sq))
```

$$k_0^2 = 0.315 \frac{32\lambda^4 t_{\text{Higgs}}^4}{g^2 t_{\text{Hubble}}^2 t_{\text{grav}}^2} = 7.887392672844198 \times 10^{-56}$$

```
In [28]: a0 = var('a0',latex_name=r"a_{0}")
expr = ((6*pi*lambdaH*g/K_EW)*t_Higgs/(t_grav^2*t_Hubble^2))^(1/3)
formula[a0] = 0.315^(1/3)*expr
pretty_print(a0,LE(r" = 0.315^{\frac{1}{3}} "),expr,'=',valof(a0))
```

$$a_0 = 0.315^{-\frac{1}{3}} \frac{6^{\frac{2}{3}}}{6 \left( \frac{\pi g \lambda t_{\text{Higgs}}}{K_{\text{EW}} t_{\text{Hubble}}^2 t_{\text{grav}}^2} \right)^{\frac{1}{3}}} = 1.3991814678093661 \times 10^{-08} s$$

```
In [29]: print_values(a0/t_Higgs)
```

$$\frac{a_0}{t_{\text{Higgs}}} = 2.6592893046343716 \times 10^{18}$$

```
In [30]: print_values(a0/a_EW)
```

$$\frac{a_0}{a_{\text{EW}}} = 4.542576387461597 \times 10^{18}$$

```
In [31]: print_values(t_Hubble^2/a0^2)
```

$$\frac{t_{\text{Hubble}}^2}{a_0^2} = 1.0706147161725437 \times 10^{51}$$

## 5.2 $w_{\text{CGF}} = 0$

```
In [32]: w_CGF = phat_CGF/rhohat_CGF
pretty_print(LE(r"w_{CGF} = "),w_CGF +O(k^4))
```

$$w_{\text{CGF}} = \left( \frac{3}{64} g^2 \left( \frac{8}{g^2} - \frac{1}{\lambda^2} \right) \right) k^2 + O(k^4)$$

```
In [33]: print_values(K_EW/(2*pi*g*lambdaH))
```

$$\frac{K_{\text{EW}}}{2 \pi g \lambda} = 0.8895346543935904$$

## 5.3 The CGF in the present

```
In [34]: omega_W = var('omega_W', latex_name=r"\omega_W")
formula[omega_W] = g/(2*lambdaH*t_Higgs)
print_values(omega_W,m_W/hbar)
```

$$\omega_W = \frac{g}{2 \lambda t_{\text{Higgs}}} = \frac{1.221171982678596 \times 10^{26}}{s} \quad \frac{m_W}{\hbar} = \frac{1.221171982678596 \times 10^{26}}{s}$$

```
In [35]: print_values(2*pi/omega_W)
```

$$\frac{2 \pi}{\omega_W} = 5.145209189452289 \times 10^{-26} s$$

```
In [36]: k0 = var('k0', latex_name=r"k_{0}")
formula[k0] = sqrt(k0sq)
print_values(k0)
print('\n')
print_values(k0*omega_W,k0*m_W)
```

$$k_0 = \sqrt{k_0^2} = 2.8084502261646374 \times 10^{-28}$$

$$k_0 \omega_W = \frac{0.03429600730939622}{s} \quad k_0 m_W = 2.257404207288874 \times 10^{-26} \text{ GeV}$$

## 5.4 CGF equation of state

```
In [37]: rho_b = var('rho_b ', latex_name=r"\rho_{b}")
formula[rho_b] = hbar/t_Higgs^4
pretty_print(rho_b, " = ", formula[rho_b] , " = ", kg*valof(rho_b/kg)/c_mps^3)
```

$$\rho_b = \frac{\hbar}{t_{\text{Higgs}}^4} = \frac{5.682491786274889 \times 10^{28} \text{ kg}}{\text{m}^3}$$

```
In [38]: rhohat_EW = var('rhohat_EW ', latex_name=r"\hat{\rho}_{EW}")
formula[rhohat_EW] = 8*K_EW^4/(3*pi^2*g^2) + 1/(8*lambdaH^2)
print_values(rhohat_EW)
```

$$\hat{\rho}_{\text{EW}} = \frac{8 K_{\text{EW}}^4}{3 \pi^2 g^2} + \frac{1}{8 \lambda^2} = 7.97415392287409$$

```
In [39]: c_b = var('c_b')
formula[c_b] = 1/(2*lambdaH^2*rhohat_EW)
print_values(c_b)
```

$$c_b = \frac{1}{2\lambda^2 \hat{\rho}_{EW}} = 0.24289366755876735$$

```
In [40]: c_a = var('c_a')
formula[c_a] = 2*lambdaH^2*(8*lambdaH^2-g^2)/(2*g^2)
c_a_val = valof(c_a)
print_values(c_a)
print(c_a_val)
```

$$c_a = -\frac{(g^2 - 8\lambda^2)\lambda^2}{g^2} = 0.9924810876684255$$

0.9924810876684255

## 5.5 Adiabatic condition for $a \geq a_{EW}$

```
In [41]: y=var('y', latex_name=r"4K_{\mathrm{EW}}(a^2H^2+\epsilon^2)^{1/2}_{\mathrm{EW}}")
formula[y] = 4*K_EW*ahat_EW*sqrt((t_grav^2/t_Higgs^2)*rhohat_EW/3+ Omega_Lambda*(t_Higgs^2/t_Hubble^2))
print_values(y)
```

$$4K_{EW}(a^2H^2 + \epsilon^2)^{1/2}_{EW} = 4K_{EW}\hat{a}_{EW}\sqrt{\frac{\Omega_{\Lambda}t_{Higgs}^2}{t_{Hubble}^2} + \frac{\hat{\rho}_{EW}t_{grav}^2}{3t_{Higgs}^2}} = 3.6360755535373564 \times 10^{-16}$$

```
In [42]: print_values((pi^2/(2*lambdaH^2))*(t_grav^2/t_Higgs^2),\
(16*pi^2*lambdaH^2/g^2)*Omega_Lambda*(t_Higgs^2/t_Hubble^2))
```

$$\frac{\pi^2 t_{grav}^2}{2\lambda^2 t_{Higgs}^2} = 5.044311146293211 \times 10^{-32} \quad \frac{16\pi^2 \Omega_{\Lambda} \lambda^2 t_{Higgs}^2}{g^2 t_{Hubble}^2} = 8.651976825635332 \times 10^{-87}$$

```
In [43]: K0 = var('K0', latex_name=r"K_{0}")
formula[K0] = pi/2
alpha0 = var('alpha0', latex_name=r"\alpha_{0}")
formula[alpha0] = (3*pi*k0sq/(2*K_EW))^(1/3)
print_values(4*K0*alpha0*a0*H0, (2*pi*lambdaH/g)*(t_Higgs/t_Hubble))
```

$$4H_0K_0a_0\alpha_0 = 1.1238604496607828 \times 10^{-43} \quad \frac{4\pi\lambda t_{Higgs}}{gt_{Hubble}} = 1.1238604496607786 \times 10^{-43}$$

## 6.4 Temperature after $a_{EW}$

```
In [44]: binary_precision=668
Reals = RealField(binary_precision)
RealNumber = Reals
myR = Reals
```

```
In [45]: Kp0 = var('Kp0', latex_name=r"K'_{0}")
value[Kp0] = elliptic_kc(1-myR(valof(k0sq)))
print_values(Kp0)
```

$$K'_0 = 64.82604415468899$$

```
In [46]: T_CGF0 = var('T_CGF0', latex_name=r"T_{\mathrm{CGF},0}")
formula[T_CGF0] = hbar/(kB*4*Kp0*alpha0*a0)
```



```

value
print_values(T_CGF0)
pretty_print("\n\n",T_CGF0," = ","%e"%(valof(T_CGF0/K))," K")
print_values(T_CGF0*kB)

```

$$T_{\text{CGF},0} = \frac{\hbar}{4 K'_0 a_0 \alpha_0 k_B} = 3597163664137.4536 K$$

$$T_{\text{CGF},0} = 3.597164\text{e}+12 \text{ K}$$

$$T_{\text{CGF},0} k_B = 0.3099795809235172 \text{ GeV}$$

```

In [47]: print_values(hbar*g/(kB*8*lambdaH*t_Higgs))

```

$$\frac{g\hbar}{8 k_B \lambda t_{\text{Higgs}}} = 233189890523018.44 K$$

```

In [48]: print_values(hbar*g/(8*lambdaH*t_Higgs))

```

$$\frac{g\hbar}{8 \lambda t_{\text{Higgs}}} = 20.09475 \text{ GeV}$$

```

In [49]: print_values(hbar*g/(kB*8*lambdaH*a0))

```

$$\frac{g\hbar}{8 a_0 k_B \lambda} = 8.768880095769793 \times 10^{-05} K$$

## 6.7 Semiclassical approximation

```

In [50]: epsilon = var('epsilon', latex_name=r"\epsilon")
value[epsilon] = 1e-27
print_values(2*pi^2*2*K_EW/(2*pi*epsilon^3*g^2))

```

$$\frac{2 \pi K_{\text{EW}}}{\epsilon^3 g^2} = 2.7327966956656648 \times 10^{82}$$
