# Supplementary material for: A theory of the dark matter
Source: arXiv:2203.12405 ancillary file (2022-03-24)
Supplement: Supplementary file 2 [file Graphs.pdf]

# Graphs

This SageMath notebook plots numerical calculations for the paper *A theory of the dark matter*.

The section numbering follows the paper. Equation numbers refer to equations in the paper.

## Preamble

```
In [1]: %display latex
LE = lambda latex_string: LatexExpr(latex_string);
```

```
In [2]: from mpmath import mp
from mpmath import mpf, mpc
import sage.libs.mpmath.all as a
mp.pretty = True
mp.dps=400
#
binary_precision=mp.prec
Reals = RealField(binary_precision+10)
RealNumber = Reals
myR = Reals
```

```
In [3]: lambdaH = var('lambdaH', latex_name=r"\lambda_H")
gsq = var('gsq', latex_name=r"g^2")
K_EW = var('K_EW', latex_name=r"K_{\mathrm{EW}}")
ahat_EW = var('ahat_EW', latex_name=r"\hat a_{\mathrm{EW}}")
m = var('m')
#m = var('m', latex_name=r"k^2")
K = var('K')
EoverK = var('EoverK', latex_name=r"\frac{E}{K}")
```

```
In [4]: lambdaH_val = 0.5080829235055462
gsq_val = 0.4262847210445738
K_EW_val = myR(mpf(1/2))
ahat_EW_val = myR(sqrt(6*pi)/(4*K_EW_val))
```

```
In [5]: Kdot = K*(EoverK/(1-m) -1)/2
EoverKdot = EoverK -1/2 -EoverK^2/(2*(1-m))
def dot(fn):
    return m*fn.derivative(m) + Kdot*fn.derivative(K) + EoverKdot*fn.derivative(EoverK)
```

```
In [6]: #
latex_name={}
latex_name['alpha'] = r"\alpha"
latex_name['bsq'] = r"\langle b^2\rangle"
latex_name['musq'] = r"\mu^2"
latex_name['ECGF'] = r"E_{\mathrm{EW}}"
latex_name['ahatsq'] = r"\hat a^2"
latex_name['rhohat'] = r"\hat \rho"
latex_name['ahat'] = r"\hat a"
latex_name['phat'] = r"\hat p"
latex_name['ahat_norm'] = r"\frac{\hat a}{\hat a_{\mathrm{EW}}}"
latex_name['phisq_norm'] = r"\frac{(\phi^\dagger\phi)_0}{v^2/2}"
latex_name['w'] = r"w"
for vstr, form in latex_name.items():
    var(vstr, latex_name=latex_name[vstr])
#
```

```
In [7]: formula={}
formula['alpha'] = ((K/K_EW)*2*(1-m+(2*m-1)*EoverK))^(1/3)
formula['bsq'] = (m-1+EoverK)/alpha^2
formula['musq'] = (1-2*m)/alpha^2
formula['ECGF'] = (m*(1-m)/2)/alpha^4
formula['ahatsq'] = 3*bsq/2 + (4*lambdaH^2/gsq)*musq
formula['rhohat'] = ((3/gsq)*ECGF+(9/(32*lambdaH^2))*bsq^2)/ahatsq^2
formula['phat'] = ((1/gsq)*(ECGF-musq*bsq)-(9/(32*lambdaH^2))*bsq^2)/ahatsq^2
formula['w'] = phat/rhohat
```

```

formula['ahat']      = (ahatsq)^(1/2)
formula['ahat_norm'] = ahat/ahat_EW
formula['phisq_norm'] = 1 - (3/2)*bsq/ahatsq
for vstr,form in formula.items():
    pretty_print(LE(latex_name[vstr]),' = ', formula[vstr], hold=True)
print('\n')

```

$$\alpha = 2^{\frac{1}{3}} \left( \frac{\left( \frac{E}{K} (2m-1) - m + 1 \right) K}{K_{EW}} \right)^{\frac{1}{3}}$$

$$\langle b^2 \rangle = \frac{\frac{E}{K} + m - 1}{\alpha^2}$$

$$\mu^2 = -\frac{2m-1}{\alpha^2}$$

$$E_{EW} = -\frac{(m-1)m}{2\alpha^4}$$

$$\hat{a}^2 = \frac{4\lambda_H^2\mu^2}{g^2} + \frac{3}{2}\langle b^2 \rangle$$

$$\hat{\rho} = \frac{3\left(\frac{32E_{EW}}{g^2} + \frac{3\langle b^2 \rangle^2}{\lambda_H^2}\right)}{32\hat{a}^2}$$

$$\hat{p} = -\frac{\frac{32(\langle b^2 \rangle \mu^2 - E_{EW})}{g^2} + \frac{9\langle b^2 \rangle^2}{\lambda_H^2}}{32\hat{a}^2}$$

$$w = \frac{\hat{p}}{\hat{\rho}}$$

$$\hat{a} = \sqrt{\hat{a}^2}$$

$$\frac{\hat{a}}{\hat{a}_{EW}} = \frac{\hat{a}}{\hat{a}_{EW}}$$

$$\frac{(\phi^\dagger \phi)_0}{v^2/2} = -\frac{3\langle b^2 \rangle}{2\hat{a}^2} + 1$$

In [8]:

```

alpha      = ((K/K_EW)*2*(1-m+(2*m-1)*EoverK))^(1/3)
bsq        = (m-1+EoverK)/alpha^2
musq       = (1-2*m)/alpha^2
ECGF       = (m*(1-m)/2)/alpha^4
ahatsq     = 3*bsq/2 + (4*lambdaH^2/gsq)*musq
rhatat     = ((3/gsq)*ECGF+(9/(32*lambdaH^2))*bsq^2)/ahatsq^2
phat       = ((1/gsq)*(ECGF-bsq*musq)-(9/(32*lambdaH^2))*bsq^2)/ahatsq^2
w          = phat/rhatat

```

```
ahat      = (ahatsq)^(1/2)
ahat_norm = ahat/ahat_EW
phisq_norm = 1 - (3/2)*bsq/ahatsq
```

```
In [9]: def paramsub(vstr):
temp = eval(vstr).subs(lambdaH=lambdaH_val,gsq=gsq_val,ahat_EW=ahat_EW_val,K_EW=K_EW_val)
return temp
```

```
In [10]: #
          alphan          = paramsub('alpha')
          bsqn            = paramsub('bsq')
          musqn           = paramsub('musq')
          ECGFn           = paramsub('ECGF')
          ahatsqn         = paramsub('ahatsq')
          rhohatn         = paramsub('rhohat')
          phatn           = paramsub('phat')
          wn              = paramsub('w')
          ahatn           = paramsub('ahat')
          ahatsqn         = paramsub('ahat_norm')
          phisq_normn     = paramsub('phisq_norm')
```

```
In [11]: def msub(v,m_val):
# # v is one of the physical variables, m is a Sage real
#     m_mpf = mpf(m_val)
m_R = myR(m_val)
K_val = myR(elliptic_kc(m_R))
E_val = myR(elliptic_ec(m_R))
EoverK_val = E_val/K_val
#     print(RDF(m_R),RDF(EoverK_val-1), RDF(E_val-K_val),RDF(K_val-myR(pi)/2))
temp = v.subs({EoverK:EoverK_val,m:m_R,K:K_val})
return myR(temp)
def fn(v):
return lambda marg: msub(v,marg)
```

```
In [12]: t = var('t')
          ahat_t = lambda t: fn(ahat_normn)(10^(-t)/2)
          w_t = lambda t: fn(w_n)(10^(-t)/2)
          phisq_t = lambda t: fn(phisq_normn)(10^(-t)/2)
          #
          plt1 = parametric_plot([ahat_t, w_t], (t, 0, 56), scale="semilogx")
          plt2 = parametric_plot([ahat_t, phisq_t], (t, 0, 56), scale="semilogx")
```

```
In [13]: anorm=var('anorm')
          coeff_low = ahat_EW_val^4 * gsq_val/(lambdaH_val^2)
          w_low = lambda anorm: -1/4/(3+anorm^4*coeff_low)
          plt3=plot(w_low,(anorm,1e-2,1),scale='semilogx')
```

```
In [14]: plt=plt1+plt2+plt3
# +line([1e-2,1),(100,1)],linestyle=":")\
plt = plt\
+text(r"$w_{\mathrm{CGF}}$", (6e1,.1),fontsize=16,color='black')\
+text(r"$\frac{\phi^\dagger\phi}{v^2/2}$", (5e1,.75),fontsize=16,color='black')\
+text(r"the Standard Model epoch", (10^3,-.3),fontsize=16,color='black',\
horizontal_alignment='left',fontweight=300)\
+text(r"$a_0$", (4.54e18,-.14),fontsize=16,color='black')\
+text(r"$a_{\mathrm{EW}}$", (1,-.14),fontsize=16,color='black')
#plt.set_aspect_ratio(1)
plt.set_axes_range(xmin=10^(-2),xmax=10^(22),ymin=0)
plt = plt+ arrow((.1,-.2),(10^21,-.2),width=1,arrowsize=2,color='black')
plt.axes_labels([r"$\frac{a}{a_{\mathrm{EW}}}$", ""])
plt.axes_labels_size(2)
#plt.axes_labels(["", ""])
show(plt,title="Figure 1",\
ticks=[[10^(-2),1,10^2,10^4,10^6,10^8,10^(10),10^(12),10^(14),10^(16),10^(18),RDF(1.0e20)], [0,1,
tick_formatter='latex')
plt.save('plots/SMepoch.pdf',dpi=600,\
ticks=[[10^(-2),1,10^2,10^4,10^6,10^8,10^(10),10^(12),10^(14),10^(16),10^(18),RDF(1.0e20)], [0,1,
tick_formatter='latex')
```

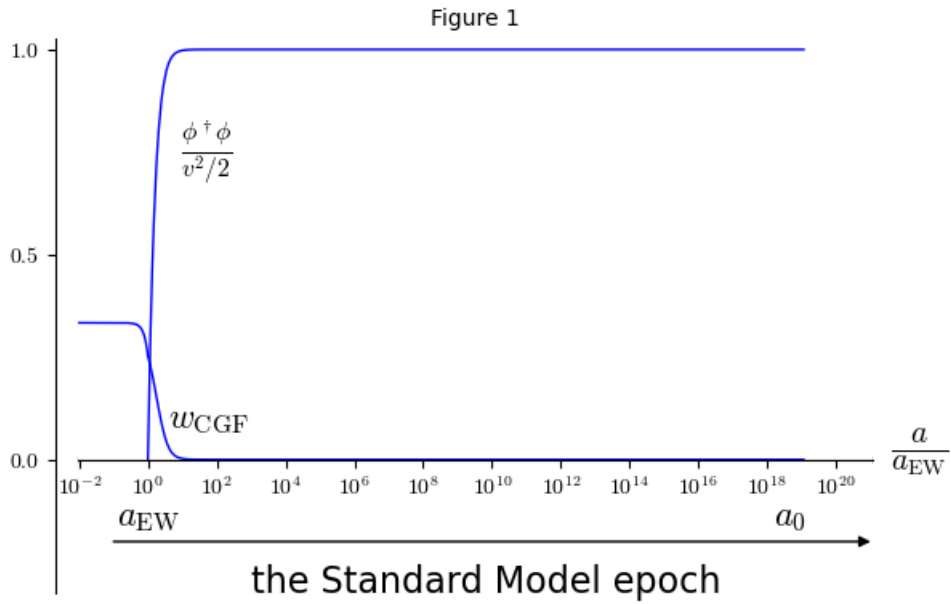

### 4.3 $a$ as a function of $k^2$

Figure 1 showing that  $a$  increases monotonically from  $a_{EW}$  to  $\infty$  as  $k^2$  decreases from  $\frac{1}{2}$  to 0.

```
In [15]: y=-(dot(ahatsq)/ahatsq)
         yn = paramsub('y')
```

```
In [16]: plt=plot(fn(yn),m,1e-8,0.5)
```

```
In [17]: plt.set_axes_range(ymin=0)
         plt.set_aspect_ratio(0.1)
         plt.axes_labels([r"$k^2$", r"$-\frac{d \ln a}{d \ln k}$"])
         plt.axes_labels_size(2)
         show(plt,title="Figure 2a")
         plt.save('plots/aofkmonotonic.pdf',dpi=600)
```

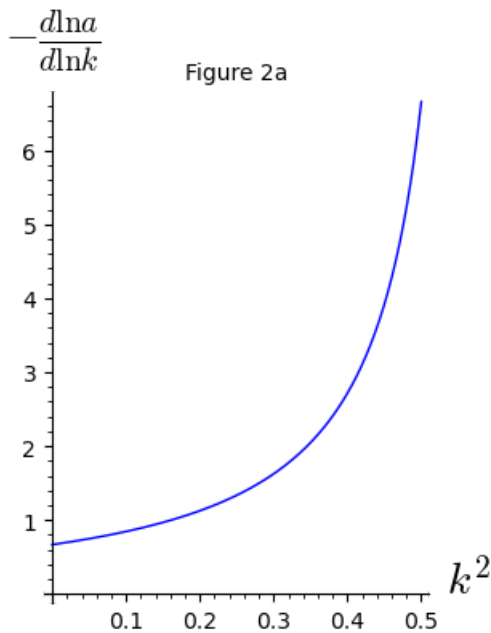

```
In [18]: plt = parametric_plot([fn(ahat_normn),m],(m,1e-5,0.5),scale="loglog")
```

```
In [19]: plt.set_aspect_ratio(0.5)
         plt.set_axes_range(xmin=1,xmax=100,ymax=0.5)
         plt.axes_labels([r"$\frac{a}{a_{\mathrm{EW}}}$", r"$k^2$"])
         plt.axes_labels_size(2)
```

```
plt.show(title="Figure 2b")
plt.savefig('plots/ksqofa.pdf',dpi=600)
```

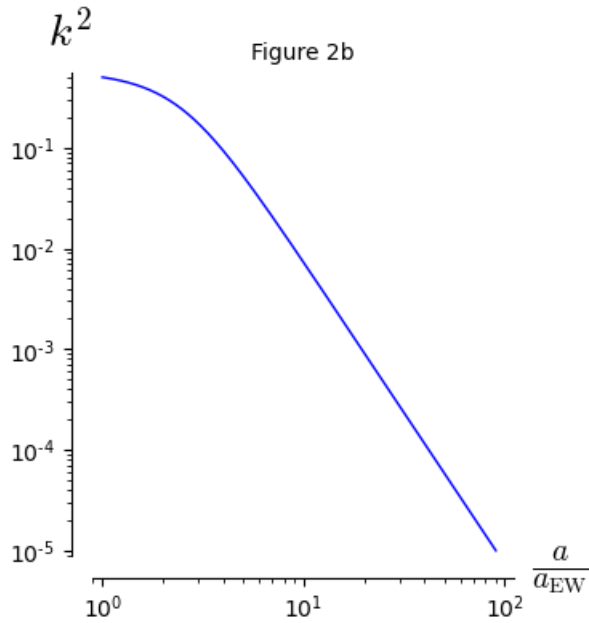

## 5.2 $w_{\text{CGF}}=0$

Figure 2 shows  $w_{\text{CGF}}$  and the progress of the electroweak transition in the first 2 ten-folds of expansion after  $a_{\text{EW}}$ .

```
In [20]: plt1 = parametric_plot([fn(ahat_normn),fn(wn)],(m,1e-6,0.5),scale="semilogx")
plt2 = parametric_plot([fn(ahat_normn),fn(phisq_normn)],(m,1e-6,0.5),scale="semilogx")
```

```
In [21]: plt=plt1+plt2\
+line([(1,1),(100,1)],linestyle=":")\
+text(r"$w_{\mathrm{CGF}}$", (2.2,.2), fontsize=16, color='black')\
+text(r"$\frac{(\phi^\dagger\phi)_0}{v^2/2}$", (2.8,.7), fontsize=16, color='black')
plt.set_aspect_ratio(1)
plt.set_axes_range(xmin=1,xmax=100)
plt.axes_labels([r"$\frac{a}{a_{\mathrm{EW}}}$", ""])
plt.axes_labels_size(2)
show(plt,title="Figure 3")
plt.savefig('plots/wandphisq.pdf',dpi=600)
```

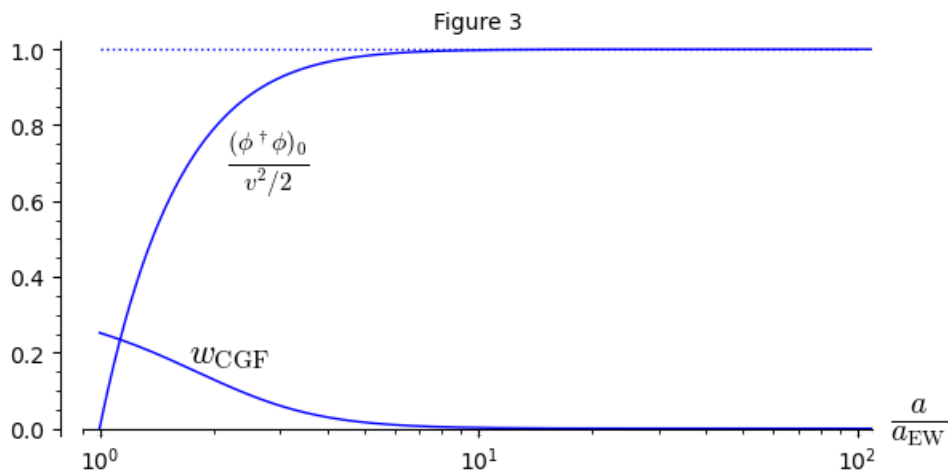

## 5.4 CGF equation of state

```
In [22]: y=(dot(rhohat)/rhohat)
yn = paramsub('y')
```

```
In [23]: plt=plot(fn(yn),m,1e-8,0.5)
```

```
In [24]: plt.set_axes_range(ymin=0)
plt.set_aspect_ratio(0.05)
plt.axes_labels([r"$k^2$", r"$\frac{d \ln \hat{\rho}_{CGF}}{d \ln k}$"])
plt.axes_labels_size(2)
show(plt, title="Figure 4")
plt.save('plots/rhoofkmonotonic.pdf', dpi=600)
```

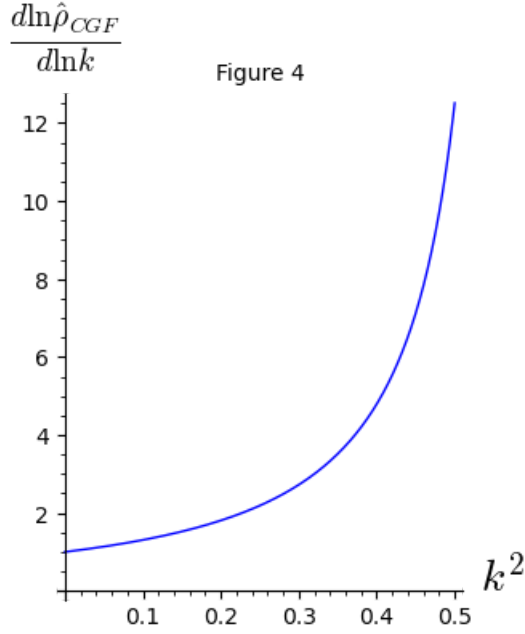

## 5.5 Adiabatic condition for $a \geq a_{EW}$

Figure 4 showing a bound on the ratio of time scales, verifying the adiabatic condition.

```
In [25]: r_gH= 2.6387686437244608e-33
r_HH= 1.3207956122976951e-88
Omega_Lambda = 0.685
pretty_print(LE(r"r_{\mathrm{gH}}=\frac{t_{\mathrm{grav}}^2}{t_{\mathrm{Higgs}}^2}=", \
RDF(r_gH), LE(r"\quad r_{\mathrm{HH}}=\frac{t_{\mathrm{Higgs}}^2}{t_{\mathrm{Hubble}}^2}=", \
LE(r"\quad \Omega_{\Lambda}="), RDF(Omega_Lambda))
```

$$r_{gH} = \frac{t_{\text{grav}}^2}{t_{\text{Higgs}}^2} = 2.6387686437244608 \times 10^{-33} \quad r_{HH} = \frac{t_{\text{Higgs}}^2}{t_{\text{Hubble}}^2} = 1.3207956122976951 \times 10^{-88} \quad \Omega_{\Lambda} = 0.685$$

```
In [26]: bound = 4*K*alpha*sqrt(r_gH*ahatsq*rhohat/3 + r_HH*Omega_Lambda*ahatsq)
boundn = paramsub('bound')
```

```
In [27]: plt= parametric_plot((fn(ahat_normn), fn(boundn)), (m, 5e-7, 0.5), scale="loglog")
```

```
In [28]: plt.set_aspect_ratio(.5)
plt.set_axes_range(ymax=1e-15, ymin=1e-19)
plt.axes_labels([r"$\frac{a}{a_{\mathrm{EW}}}$", r"$y$"])
plt.axes_labels_size(2)
show(plt, title="Figure 5")
plt.save('plots/adiabaticbound.pdf', dpi=600)
```

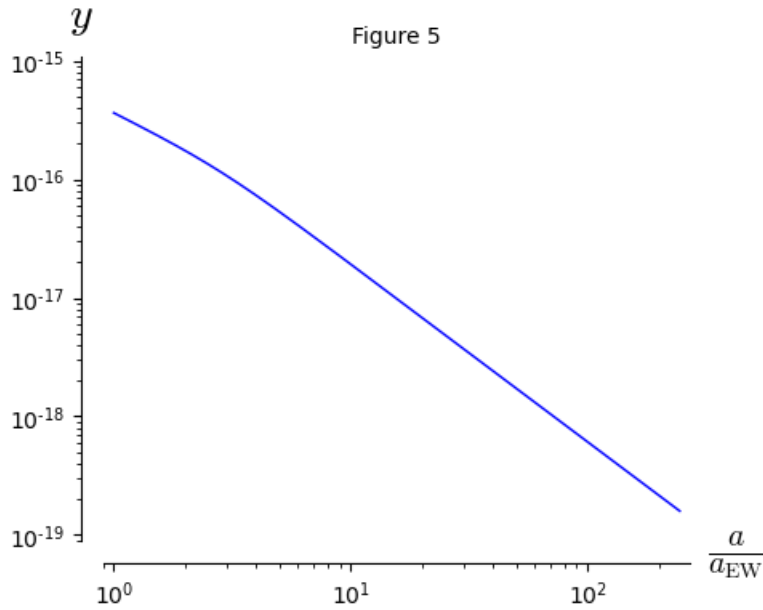

## 6.4 Temperature after $a_{EW}$

CGF temperature  $k_B T_{CGF} = \frac{\hbar}{4K'\alpha a} = \frac{m_{Higgs}}{4K'\alpha \hat{a}}$

redshifted to the present  $k_B T_{rs} = \frac{a}{a_0} k_B T_{CGF} = \frac{m_{Higgs}}{4K'\alpha \hat{a}_0}$

use numbers from the Arithmetic notebook and from above

In [29]:

```
T_CMB = mpf(2.7255) # K
K_EW_mpf = mp.ellipk(1/2)
m_Higgs_mpf = mpf(125.1) # GeV
kB_mpf = mpf(8.61733326214518e-14) # GeV/K
ahat0_mpf = mpf(2.6592893046343716e18) # s
ahat_EW_mpf = mpf(0.5854143283037644) # s
lambda_mpf = mpf(lambdaH_val)
gsq_mpf = mpf(gsq_val) # g^2
```

define functions in mpmath

In [30]:

```
def kT_CGF(ma):
    m=mpf(ma)
    K = mp.ellipk(m)
    Kp = mp.ellipk(1-m)
    E = mp.ellipe(m)
    EoverK = E/K
    alpha = mp.power( (K/K_EW_mpf)*2*(1-m+(2*m-1)*EoverK) , 1/3)
    ahatsq = ((3/2)*(m-1+EoverK)+(4*lambda_mpf^2/gsq_mpf)*(1-2*m))/alpha^2
    ahat = mp.sqrt(ahatsq)
    return m_Higgs_mpf/(4*Kp*alpha*ahat)

def T_rs(ma):
    m=mpf(ma)
    K = mp.ellipk(m)
    Kp = mp.ellipk(1-m)
    E = mp.ellipe(m)
    EoverK = E/K
    alpha = mp.power( (K/K_EW_mpf)*2*(1-m+(2*m-1)*EoverK) , 1/3)
    return m_Higgs_mpf/(4*Kp*alpha*ahat0_mpf*kB_mpf)

def ahat_over_ahat0_mp(ma):
    m=mpf(ma)
    K = mp.ellipk(m)
    E = mp.ellipe(m)
    EoverK = E/K
    alpha = mp.power( (K/K_EW_mpf)*2*(1-m+(2*m-1)*EoverK) , 1/3)
    ahatsq = ((3/2)*(m-1+EoverK)+(4*lambda_mpf^2/gsq_mpf)*(1-2*m))/alpha^2
    ahat = mp.sqrt(ahatsq)
    return ahat/ahat_EW_mpf
```

In [31]:

```
plt=parametric_plot((ahat_over_ahat0_mp,kT_CGF),(m,1e-21,0.5),scale="semilogx")
plt.set_aspect_ratio(.1)
plt.set_axes_range(ymin=0,ymax=30,xmin=1,xmax=1e7)
```

```

yaxis_label = Graphics()+text(r"$ k_{\mathrm{B}} T_{\mathrm{CGF}}$",(-0.15,0.80),axis_coords=True,font:
yaxis_label += text(r"$ (\mathrm{GeV})$",(-0.15,0.70),axis_coords=True,fontsize=11,color='black')
xaxis_label = Graphics()+text(r"$\frac{a}{a_{\mathrm{EW}}}$", (1.05,-0.04),axis_coords=True,fontsize=11,color='black')
plt2 = plt+yaxis_label+xaxis_label
plt2.axes_labels_size(2)
show(plt2,title="Figure 6",figsize=[8,20],ymax=30,xmin=1)
plt2.save('plots/kT_after_a_EW.pdf',figsize=[8,20],ymax=30,xmin=1,dpi=600)

```

Figure 6

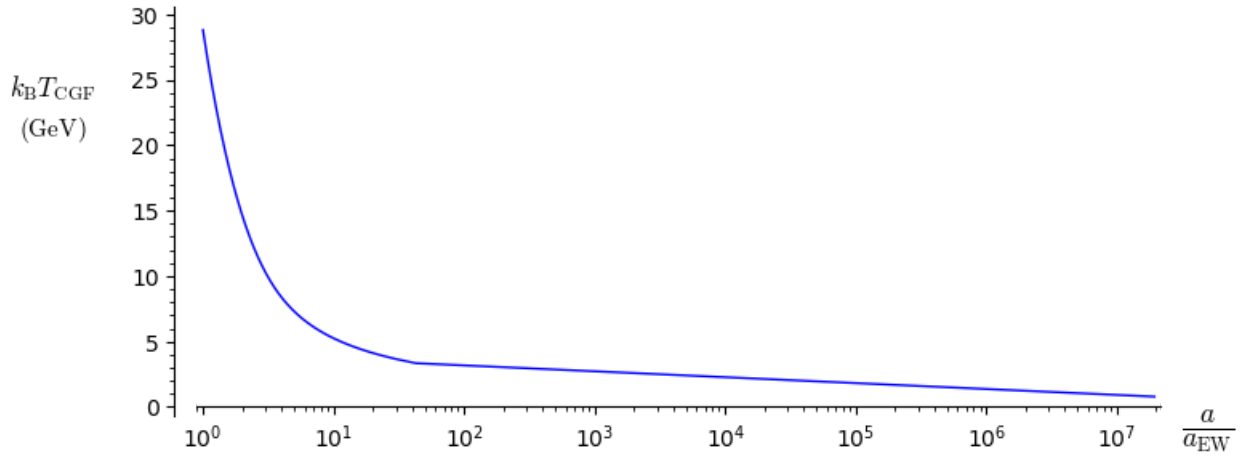

Solve  $T_{\mathrm{rs}}(k^2) = T_{\mathrm{CMB}}$

```

In [32]: m_dc=mp.findroot(lambda ma: T_rs(ma)-T_CMB,1e-17,solver='newton')
T_rs_dc=T_rs(m_dc)
ahatnorm_dc = ahat_over_ahat0_mp(m_dc)
kT_dc = kT_CGF(m_dc)

```

```

In [33]: pretty_print(\
    LE(r"k^2 = "), RDF(m_dc).n(prec=20), \
    LE(r"\quad \frac{a}{a_0} k_{\mathrm{B}} T_{\mathrm{CGF}} = "), RDF(T_rs_dc).n(prec=20), LE(r"\, \mathrm{K}"), \
    LE(r"\quad \frac{a}{a_0} = "), RDF(ahatnorm_dc).n(prec=20), \
    LE(r"\quad k_{\mathrm{B}} T_{\mathrm{CGF}} = "), RDF(kT_dc).n(prec=20), LE(r"\, \mathrm{GeV}"))

```

$$k^2 = 5.1168 \times 10^{-18} \quad \frac{a}{a_0} k_{\mathrm{B}} T_{\mathrm{CGF}} = 2.7255 \text{ K} \quad \frac{a}{a_0} = 1.1305 \times 10^6 \quad k_{\mathrm{B}} T_{\mathrm{CGF}} = 0.94371 \text{ GeV}$$
